# Supplementary material for: Closing of the Induced Gap in a Hybrid Superconductor-Semiconductor Nanowire
Source: arXiv:2006.01275 source file (2020-06-01)
Supplement: Supplementary file 1 [file supplement.pdf]

# Supplement to "Closing of the Induced Gap in a Hybrid Superconductor-Semiconductor Nanowire"

D. Puglia,[1,2] E. A. Martinez,[1] G. C. Ménard,[1] A. Pöschl,[1] S. Gronin,[3] G. C. Gardner,[3] R. Kallaher,[3] M. J. Manfra,[3,4,5,6] C. M. Marcus,[1] A. P. Higginbotham,[1,2,*] and L. Casparis[1,†]

[1]*Microsoft Quantum Labs Copenhagen and Center for Quantum Devices, Niels Bohr Institute, University of Copenhagen, Universitetsparken 5, 2100 Copenhagen, Denmark*
[2]*Institute of Science and Technology Austria, Am Campus 1, 3400 Klosterneuburg, Austria*
[3]*Microsoft Quantum Purdue, and Birck Nanotechnology Center, Purdue University, West Lafayette, IN, USA*
[4]*Department of Physics and Astronomy, Purdue University, West Lafayette, IN, USA*
[5]*School of Materials Engineering, Purdue University, West Lafayette, IN, USA*
[6]*School of Electrical and Computer Engineering, Purdue University, West Lafayette, IN, USA*

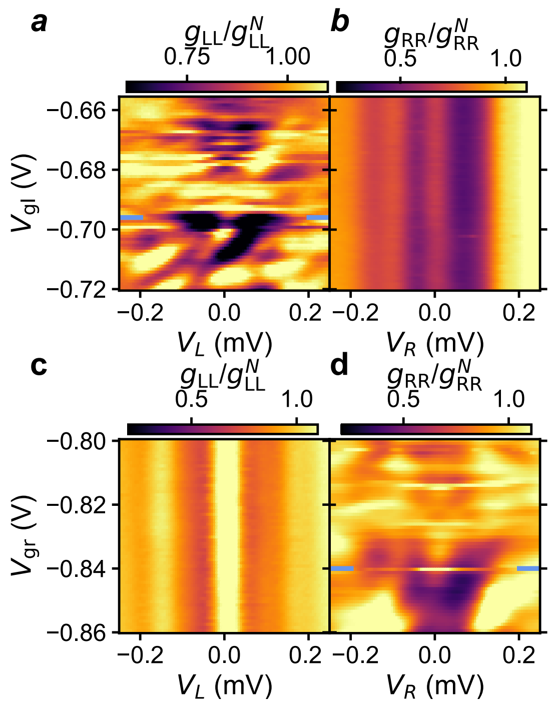


FIG. S1. Tunnel-barrier dependence of local conductance at $B = 0.7$ T. **a** (**b**) Local conductance $g_{\rm LL}$ ($g_{\rm RR}$) normalized by conductance at high bias $g^N_{\rm LL}$ ($g^N_{\rm RR}$) measured as a function of bias voltage and left tunnel-barrier $V_{\rm gl}$, while $V_{\rm gr} = -0.84$ V. **c** (**d**) $g_{\rm LL}$ ($g_{\rm RR}$) normalized by conductance at high bias $g^N_{\rm LL}$ ($g^N_{\rm RR}$) as a function of bias and right tunnel-barrier $V_{\rm gr}$, while $V_{\rm gl} = -0.696$ V. The blue markers indicate the tunnel-barrier values for the field and plunger dependence presented in Figure 4 of the main text, $V_{\rm gl} = -0.696$ V and $V_{\rm gr} = -0.84$ V.

## TUNNEL BARRIER SCANS

Figure S1 shows the dependence of the local conductances $g_{\rm LL}$ and $g_{\rm RR}$ on the left and right tunnel barriers at a magnetic field $B = 0.7$ T. The conductance data are normalized to the high bias values $g^N_{\rm LL} = g_{\rm LL}(220\mu eV)$ for every cutter gate voltage. This is done to allow for comparison of the data in a large range of conductance values. $g^N_{\rm LL}$ ranges from $\sim 1.2\ \frac{e^2}{h}$ to pinch off in Fig. S1a. $g^N_{\rm RR}$ ranges from $\sim 0.8\ \frac{e^2}{h}$ to pinch off in Fig. S1d. Local conductance on the left and right show many resonances as function of tunnel gate [Fig. S1a and Fig.S1d]. Zero-bias peaks appear frequently, and are typically present for a few-tens of millivolts of gate voltage. We note that the local conductance on the side with constant gate voltage is not affected [Fig. S1b and Fig.S1c] by the barrier change on the other side. This observation is consistent with changing local tunnel coupling to a robust topological phase in the middle of the

nanowire, but also with a purely local origin of the ZBPs, highlighting again the need for a technique probing the bulk of the sample.

## EXTRACTION OF $S$

Figure S2 shows how the slope of the nonlocal conductance $S$ was extracted. The first derivative for every linecut was calculated by a Savitzky-Golay filter over a bias window of $\pm$ 61  V centered around zero bias.

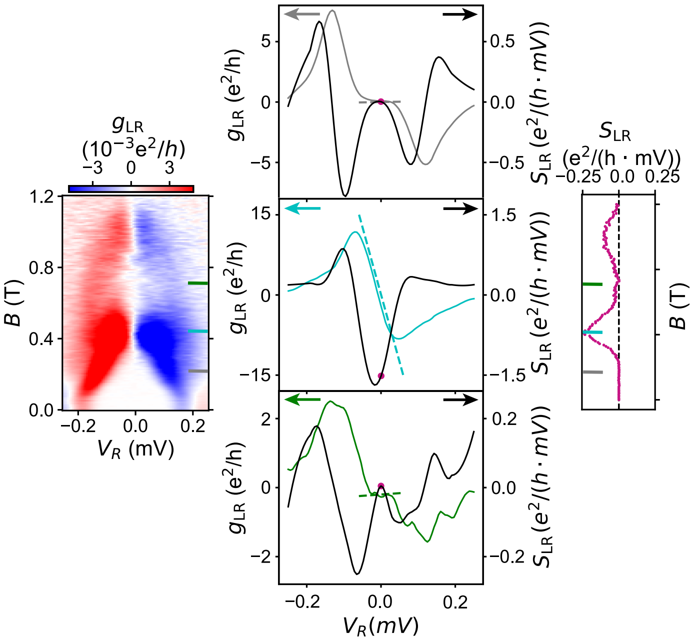


FIG. S2. Slope extraction from nonlocal conductance. The left panels shows the $g_{\mathrm{LR}}$ field scan introduced in Fig. 2d of the main text. The center panels present how the nonlocal slope $S_{\mathrm{LR}}$ was extracted for 3 values of field: 0.2 T (gray), 0.41 T (blue), and 0.71 T (green). The linecut of $g_{\mathrm{LR}}$ is shown by a continuous colored line for the respective fields. The first derivative of the linecut ($S_{\mathrm{LR}}$) was calculated by the Savitzky-Golay filter and is shown in black with the zero-bias values evidenced by a magenta dot. For reference, the value of the slope at zero-bias was multiplied by the bias voltage and displayed as a color dashed line for each linecut. The right panel presents the slope $S_{LR}$ extracted at zero-bias (magenta dot in the center panel) for the entire field scan.

## ROBUSTNESS OF THE LOW-BIAS NONLOCAL RESPONSE

In the main text, it is shown that a regime with low-bias nonlocal conductance extends over large ranges of magnetic field and several hundreds of millivolts in gate voltage, persisting even when zero-bias peaks are absent. The robustness of this regime is further demonstrated in Fig. S3. Nonlocal conductances are plotted as a function of plunger $V_p$ at three different magnetic fields. At small fields, nonlocal conductance is only observed above a characteristic bias-scale, which we operationally identify as the induced gap [Fig. S3a]. At higher field the nonlocal response is observed for low biases, although the sign and magnitude fluctuates strongly, and persists for the entire range of several volts in plunger-gate voltage [Fig. S3c and d]. For comparison, zero-bias peaks are often considered to be robust if they persist over orders-of-magnitude smaller voltage ranges using similar gating geometries [1]. Thus, low-bias nonlocal response is a large-scale feature of the dataset, and is substantially more robust than zero-bias peaks.

Figure S4 show the local conductances for the same magnetic fields and plunger range. At $B$ = 0.2 T, sub-gap features showing up only in one local conductance [Fig. S4a] are not present in the nonlocal conductance [Fig. S3a], consistent with the expectation that nonlocal conductance is insensitive to low-energy localized states when the rest of the wire is still trivially gapped. At higher magnetic fields there is a dense structure of low-bias peaks [Fig. S4b,c], with no obvious correlation to the nonlocal data.

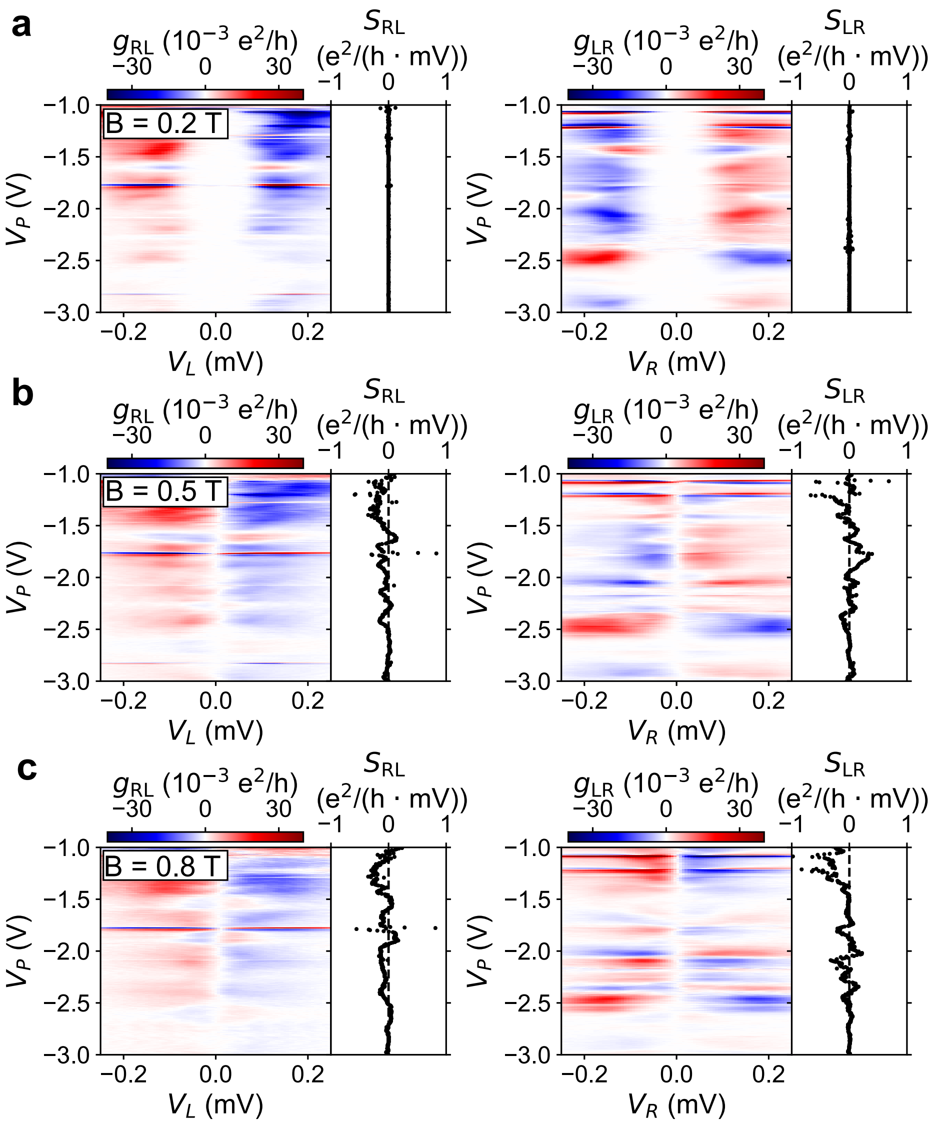


FIG. S3. **Gate-voltage dependence of the nonlocal conductance at different magnetic fields.** Nonlocal conductances $g_{\rm RL}$ and $g_{\rm LR}$ measured as a function of bias voltage and plunger gate $V_P$ taken at $B = 0.2$ T for **a**, $B = 0.5$ T for **b**, and $B = 0.8$ T for **c**. The nonlocal slope $S$ was numerically computed using the same procedure as in the main text and is shown in the right panel.

## EXAMPLE DATA FROM A SECOND DEVICE

Figure S5 shows data from a 2 $\mu$m long three-terminal device. The main features of the data are qualitatively similar to the data shown in the main text for the 1 $\mu$m device. Namely the emergence of a robust, low-energy nonlocal conductance above a critical field, as seen from the nonlocal conductance. This particular device exhibited many subgap state at zero field, including the occurrence of ZBPs in both $g_{\rm LL}$ and $g_{\rm RR}$.


* Equal contribution, andrew.higginbotham@ist.ac.at

† Equal contribution, lucas.casparis@microsoft.com



[1] M. T. Deng, S. Vaitiekėnas, E. B. Hansen, J. Danon, M. Leijnse, K. Flensberg, J. Nygård, P. Krogstrup, and C. M. Marcus, Science **354**, 1557 (2016).

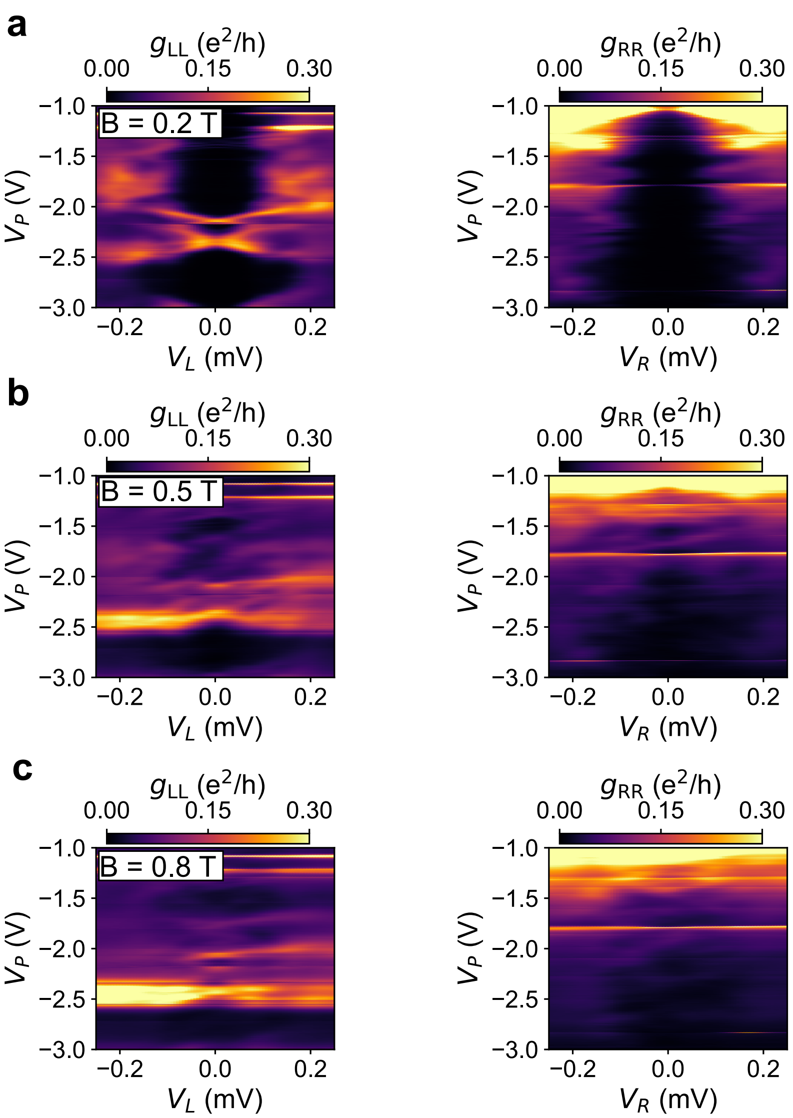


FIG. S4. **Gate-voltage dependence of the local conductance at different magnetic fields.** Local conductances $g_{\mathrm{LL}}$ and $g_{\mathrm{RR}}$ measured as a function of bias voltage and plunger gate $V_P$ taken at $B = 0.2$ T for **a**, $B = 0.5$ T for **b**, and $B = 0.8$ T for **c**. Data were taken simultaneously with nonlocal measurements in Fig. S3.

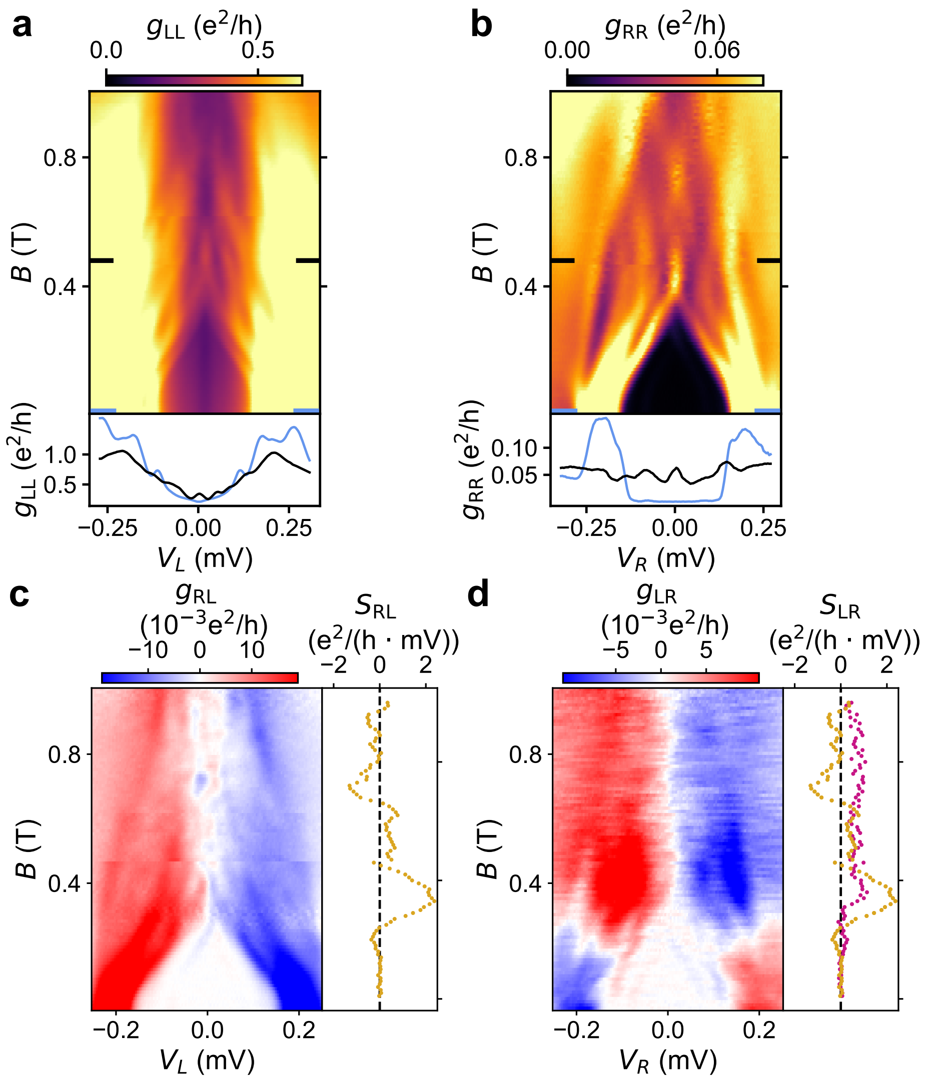


FIG. S5. **Magnetic field dependence of the full conductance matrix for a 2 $\mu$m long device.** Local conductances **a**, $g_{\rm LL}$ and **b**, $g_{\rm RR}$ measured as a function of bias voltage and magnetic field $B$, with linecuts at $B = 0$T and $B = 0.48$ T shown in the bottom panels. Nonlocal conductances **c**, $g_{\rm RL}$ and **d**, $g_{\rm LR}$ with nonlocal conductance slope $S$ shown in right panel. $S$, was numerically computed using the same procedure as in the main text. For comparison, $S_{\rm LR}$ from **c** (orange) is overlaid in **d**.
